# Supplementary material for: Fraction of $\chi_c$ decays in prompt $J/\psi$ production measured in pPb collisions at $\sqrt{s_{NN}}=8.16$ TeV
Source: arXiv:2311.01562 source file (2023-11-02)
Supplement: Supplementary file 2 [file supplementary-app.tex]

\clearpage

\section*{Supplementary material for LHCb-PAPER-2023-028}
\label{sec:Supplementary-App}

\begin{table*}[!htb]
    \centering
    \caption{Fraction of \chic decays in the prompt \jpsi yield in $p$Pb collisions. Uncertainties are statistical, systematic and from \chic polarization, respectively.}
    \label{tab:fchic_result}
    \begin{tabular}{cccc}
       $\frac{\pt}{\gevc}$  &  {\footnotesize $\frac{<\pt>}{\gevc}$} & $1.5<y^*<4.0$ & $-5.0<y^*<-2.5$ \\\hline
         1--2 & 1.5 & 0.185 $\pm$ 0.023 $\pm$ 0.025 + 0.031 & 0.277 $\pm$ 0.037 $\pm$ 0.050 + 0.050\\
         2--3 & 2.5 & 0.157 $\pm$ 0.019 $\pm$ 0.014 + 0.006 & 0.219 $\pm$ 0.022 $\pm$ 0.011 + 0.010\\
         3--4 & 3.5 & 0.168 $\pm$ 0.016 $\pm$ 0.005 + 0.007 & 0.178 $\pm$ 0.018 $\pm$ 0.016 + 0.009\\
         4--5 & 4.5 & 0.198 $\pm$ 0.015 $\pm$ 0.009 + 0.012 & 0.141 $\pm$ 0.016 $\pm$ 0.006 + 0.008\\
         5--6 & 5.5 & 0.180 $\pm$ 0.016 $\pm$ 0.005 + 0.013 & 0.164 $\pm$ 0.018 $\pm$ 0.009 + 0.011\\
         6--7 & 6.5 & 0.200 $\pm$ 0.017 $\pm$ 0.013 + 0.014 & 0.193 $\pm$ 0.020 $\pm$ 0.010 + 0.013\\
         7--10 & 8.0 & 0.235 $\pm$ 0.027 $\pm$ 0.018 $^{+0.019}_{-0.005}$ & 0.208 $\pm$ 0.023 $\pm$ 0.018 $^{+0.016}_{-0.004}$\\
         10--20 & 13.8 & 0.217 $\pm$ 0.024 $\pm$ 0.016 $^{+0.017}_{-0.007}$ & 0.274 $\pm$ 0.035 $\pm$  0.010 $^{+0.022}_{-0.008}$\\
    \end{tabular}
\end{table*}

\clearpage

\begin{figure*}[htb]
    \centering
    \includegraphics[width=1.0\linewidth]{figs/Fig4.pdf}
    \caption{Distribution of $\Delta M=M_{\mup\mun\gamma}-M_{\mup\mun}$ in the \chic mass region in different \ptjpsi intervals in the forward rapidity region $1.5<y^*<4.0$.  The lower panels show the combinatorial background-subtracted mass distributions. The red, blue and gray bands represent the total fit, the combinatorial background and the correlated background, respectively. The width of the bands corresponds to 68\% CL.}
    \label{fig:chic_peaks-pPb}
\end{figure*}

\begin{figure*}
    \includegraphics[width=1.0\linewidth]{figs/Fig5.pdf}
    \caption{Distribution of $\Delta M=M_{\mup\mun\gamma}-M_{\mup\mun}$ in the \chic mass region in different \ptjpsi intervals in the forward rapidity $-5.0<y^*<-2.5$. The lower panels show the combinatorial background-subtracted mass distributions. The red, blue and gray bands represent the total fit, the combinatorial background and the correlated background, respectively. The width of the bands corresponds to 68\% CL.}
\end{figure*}

\begin{figure*}
    \centering
    $1.5<y^*<4.0$
    \includegraphics[width=1.0\linewidth]{figs/Fig6top.pdf}
    $-5.0<y^*<-2.5$
    \includegraphics[width=1.0\linewidth]{figs/Fig6bottom.pdf}
    \caption{Invariant mass distribution of \mup\mun pairs in the \jpsi mass region in different \ptjpsi intervals. The red and gray bands correspond to the 68\% CL function fitted to the data and background contribution, respectively.}
\end{figure*}

\begin{figure*}
    \input{figs/Fig7}
    \caption{Summary of $\chic/\jpsi$ cross section ratio measurements. Results from $p$A collisions at HERA-B \cite{HERA-B:2008rhh} and $d$Au collisions at PHENIX \cite{PHENIX:2013pmn} are compared to the \lhcb results. The HERA-B $p$W points are shifted horizontally for clarity. The gray band represents the systematic uncertainty from the \chic and \jpsi polarization effects in the \lhcb results.}
    \label{fig:fchic_comparisons}
\end{figure*}

\clearpage

\begin{figure*}
    \centering
    \input{figs/Fig8}
    \caption{Double ratio $\sigma_{\chic\to\jpsi\gamma}/\sigma_{\jpsi}$ between $pp$ and $p$Pb collisions. The $pp$ reference is obtained from Ref. \cite{LHCb-PAPER-2011-030}. The error bars include statistical and systematic uncertainties.}
    \label{fig:double_ratio_rap}
\end{figure*}
